# Supplementary material for: Bitrate-Constrained DRO: Beyond Worst Case Robustness To Unknown Group Shifts
Source: arXiv:2302.02931 source file (2023-10-12)
Supplement: Supplementary file 1 [file appendix-backup.tex]

% Keeping backup for future work
{
\clearpage
\newcommand{\skw}{\Phi} % Skew sets. Need a better notation
\newcommand{\mcG}{\mathcal{G}}
\newcommand{\fr}{\mathcal{F}}
\newcommand{\mcX}{\mathcal{X}}
\newcommand{\lt}{l_{\theta}}
\newcommand{\lth}{{\hat{l}_{\theta}}}
\newcommand{\rth}{{\hat{r}_t}}

\subsection{Regret based stuff}


Main takeaways,
\begin{enumerate}
    \item Fixing a $\abs{\mcG}$, we are robust to all groups of size $\abs{\mcG}$; as robust (fair) as the uniform distribution can be.
    \item We are $O(\sqrt{\frac{\abs{\mcG}}{T}})$ close to optimal $r^*$, not necessarily corresponding to uniform. $r^*$ is implied by the constraint on the adversary. 
    \item In general if $q(r^*) = u + \eps$ for an $\eps$ biased adversarial action space, we are $\eps$ sub-optimal to the most fair classifier (risk minimization against uniform).
    \item Iterate condition option 1 - in case we want more details: Even though our algorithm is playing no-regret sub-optimally, we can still attain $O(\sqrt{T})$-subgradient optimization rate assuming some \emph{weak-learning} like conditions.
    \item All of the above is holds even if we keep on changing $\mcG$ keeping $\abs{\mcG}$ constant \emph{as long as} the adversary is also unbiased on the new action space. Controlling the adversary is critical and if we can't control the adversary uniformly over all $\set{\mcG \mid \abs{\mcG} \text{is fixed}}$, we need to quantify all above statements to all group definitions where we can constrain the adversary. For example, define $\set{\mcG_{\mathcal{A}}}$ where we can constraint the adversary (groups definition based on simple features, say). Then the above is true for all $\mcG$ in this set.
    \item Finally, for high dimensional problems $\abs{\mcG}$, the fair distribution and the `worst adversary' or the most biased adversary (i.e can only play one vertex) differs by $O(1 - \frac{1}{\sqrt{\abs{\mcG}}})$, thus making the solution kind of useless in the worst case. But again, if we have a cooperative or optimistic player 2 (unbiased adversary), we are golden.
    \item \emph{Caution:} Have not thought enough about fairness assumption.
    \item \emph{Caution:} All feelings, no verification.
    \item \emph{Maybe point:} Constraining adversary using bit-rate constraints is one way of ensuring this way of unbaisedness. There could be other ways? In particular, if we know how to construct a constrained adversary for some a set of group definitions $\set{\mcG}$, we can uniformly be as fair (as it gets) to all of them.
    \item (In the general context of any algorithm vs nature) We defined fairness with respect to uniform because we assume nature can uniformly pick over the uncertainty set. Say we want to model some $\pi$ prior for nature instead. We can do that as,
    \[
    \fr(l_\theta, q; \mcG, \pi) = \max_{G_i \in \mcG} \E_\pi\E_{q\mid\pi}[l_{\theta}] - \E_{q\mid G_i}[l_{\theta}].
    \] Setting $\pi = u$ recovers the uniform case where $\E_u \E_{q\mid u} \lt = \E_q \lt$. Moreover, if we want to get the group DRO objective out of this, put the prior on the worst-group ($\pi$ is a vertex of the simplex). Note that the constraint on the adversary also needs to respect the prior.
    
    \item Purity vector -- not $l$ vector. Purity vector is $[0, 1]$ continuous bound and not $\set{0, 1}$. Makes life easier, especially for small $\abs{\mcG}$.
    \item Note that under the uniform assumption you don't even need group information to evaluate unseen distribution performance. It will be, by definition, close to your test performance. Obviously if your test performance it self is garbage there is nothing much we can do.
    
    \item BTW, the intuition for why the dimensional dependency is $\abs{G}$ is the same as why we have a $\sqrt{k}$-separation dependency $k$-means problem in $d$ dimensions, with $d \gg k$. You'd expect a $\sqrt{d}$ separation requirement, say between two gaussians in $d$ dimension, since the gaussian annulus is concentrated at $\sqrt{d}$.  Essentially, the intuition is that the problem is unchanged under a projection onto $\abs{\mcG}$ dimension. See later \url{https://arxiv.org/abs/1206.3204}. 
\end{enumerate}

(Language will be fixed later. Arguments need work)

Notation: 
\begin{itemize}
    \item Speaking mostly on function space over $\mcX$.
    \item $l_\theta : \mcX \rightarrow \set{0, 1}$, will be loss functions indexed by model parameters $\theta \in \Theta$.
    \item $\Delta(\mcX):$ Simplex over $\mcX$, distributions over $\mcX$.
    \item $p, q$ distributions in $\Delta(\mcX)$.
    \item \emph{group definition} $\mcG: \set{G_1, \dots, G_{\abs{G}}}$, $\cup_{G_i} = \mcX$, $G_j \cap G_i = \phi $ for $i \ne j$ (partitions).
\end{itemize}

\begin{definition}[Skew distributions] For a group definition $\mcG = \set{G_1, \dots, G_{\abs{\mcG}}}$, define  
\[
    \mathrm{\skw}(\mcG; m_0, m_1, M)
    = \set{q \in \Delta(\mcX)\mid 0 < m_0 \le q(G_i) \le m_1 \ \text{or}\ q(G_i) > M \ge 0.5, \forall G_i \in \mcG}.
\]
\end{definition}

\begin{definition}[Fair model] For a group definition $\mcG$, a distribution $q$ and $l_\theta$ a $0$-$1$ loss function realized at $\theta \in \Theta$ define,
\[
    \fr(l_\theta, q; \mcG) = \max_{G_i \in \mcG} \E_{q }[l_{\theta}] - \E_{q\mid G_i}[l_{\theta}]
\]
\end{definition}
\begin{enumerate}
    \item $\fr(\cdot, q; G)$ is convex in $l$ for fixed $q$ and $G$. $l$ is convex relaxation of $\lt \in \set{0,1}$ to $ \lt \in [0, 1]$.
    \item $\fr(l, \cdot; G)$ is concave (linear) in $q$ for fixed $l$ and $G$.
\end{enumerate}

For some $q \in \Delta(\mcX)$ let $l_{\theta_{q}} = \argmin_{\theta \in \Theta}\E_{q}l_{\theta}$, the solution returned by risk minimization if we had access to distribution $q$. In particular let $u$ denote the uniform distribution.

\emph{Assumption 1: Risk minimization is fair given oracle access to $u$.} That is, for all (any) $\mcG$, $q$,
\[
 \fr(l_{\theta_u}, u; \mcG) \le \fr(l_{\theta_q}, q; \mcG).
\]

That is, if I had oracle access to the uniform distribution over $\mcX$, I can  learn the most fair model through risk minimization on $u$ and I'll be done.

Here we have not yet restricted $\fr(l_{\theta_u}, u; \mcG)$ from above so it can be quite bad in general. We just need others to be worse. TODO: Think about this. Is this too strong or reasonable? We can relax this later. At some level this is saying that the unbiased oracle is the \emph{right} oracle.

Now let a $\mcG^*$ be such that  $p \in \skw(\mcG^*; m_0, m_1, M)$. That is, we have received data from some skewed distribution with respect to some group definition (fixed for now).

Define set of group shifts around $p$ with respect to groups $\mcG$,
\[
    U_{f}(p, \delta, \mcG) = \set{q \mid D_{f}(q ||p ) \le \delta, \E_{q\mid G_i}I[G_i] = \E_{p\mid G_i} I[G_i]},
\]

\begin{enumerate}
    \item We are going to assume that there is at least one majority group in $\mcG^*$. 
    \item For any fixed $\abs{\mcG^*}$, any distribution can be projected onto $\Delta^{\abs{\mcG}}$. Note that each every group distribution is in $\abs{\mcG^*}$.
    \item For simplicity assume that $\delta = 1$. This means that the uniform distribution can be represented as a group shift. That is $u \in U_f(p, \delta, \mcG)$.
\end{enumerate}

 If thinking in terms of the re-weighting function $r$, replace $q$ with $q(r)$. We can always recover $q$ from $r$. Consider the following optimization program,

\[
    \min_{\lt \in \Theta} \max_{q \in U_f(p, 1.0, \mcG^*)} \fr(\lt, q; \mcG^*) = V^*
\] It follows from assumption $1$ that, 
$$
   V^* = \fr({\lt}_u, q_u; \mcG^*).
$$

Okay the remaining argument is as follows. We are solving,
\[
    \min_{\lt \in \Theta} \max_{q \in U_f(p, 1.0, \mcG^*)} \fr(\lt, q; \mcG^*) = V^*.
\] We know that $(l_{\theta_u}, u)$ (or $(l_{\theta_u}, u(r))$) is the equilibrium point.
Both $\min$-player and $\max$-player is playing no-regret. For concreteness, say both are running  FTRL with $\ell_2$ regularization (i.e gradient descent not SGD sadly).

Thus, at each round both players play ${\lt}_t$ and $q(r_t)$ where,
\[
    {\lt}_t = \arg\min_{\lt} \sum_{\tau=1}^{t-1} \fr(\lt, q(r_\tau); \mcG^*)\quad\text{and}\quad
    q({r}_t) = \arg\min_{q(r) \in U_f(p, 1, \mcG^*)}  \sum_{\tau=1}^{t-1} \fr({\lt}_{\tau}, q(r); \mcG^*).
\]Note that this corresponds to the descent-ascent update rule (roughly -- not being careful),
\[
    {\lt}_t = {\lt}_{t-1} - \frac{1}{\eta} \partial\sum_{\tau=1}^{t-1} \fr({\lt}_t, q(r_\tau); \mcG^*)\quad\text{and}\quad
    q({r}_t) = q(r_{t-1}) - \partial \sum_{\tau=1}^{t-1} \fr({\lt}_{\tau}, q(r_{t-1}); \mcG^*).
\]


Now of course we cannot solve this optimization over $\theta$ or $r$. Since $\theta$ requires us to solve a non-convex problem and picking $r$ requires access to $u$, which in turn requires access of $(G^*)$.

To try to work around this we are going to model $\lth = \lt + \eps(\lt)$ and $q(\rth) = q(r_t) + \eps(r_t)$. Then we are going to control $\eps(\lt)$, $\eps(r_t)$ and invoke Theorem 5.2 here: \url{https://arxiv.org/pdf/1807.04936.pdf}. We can apply the theorem directly for the max-player; they are linear in $q$ so the gradient is just $\lt$. For the min-player the gradient is not $q(\rth)$ by $q\mid{G_i}(\rth)$ for some $i$ so a little work needs to be done to bound it. I will talk about how we control $\eps(\lt)$ and $\eps(r_t)$ in a bit.

This will help us control iterates ${\lt}_t$ and $q({r}_t)$. Finally we invoke Theorem~9, here \url{http://proceedings.mlr.press/v75/abernethy18a/abernethy18a.pdf}, to complete our argument that $(\overline{\lt}, \overline{q(r_t)})$ is $O(\frac{1}{\sqrt{T}}\abs{\mcG})$-equilibrium point.

\subsubsection{Controlling $\eps(\lt)$ and $\eps(r_t)$}

Rough arguments:
\begin{itemize}
\item Project everything onto $\Delta^{\mcG - 1}$ using the group conditional projection with a fixed group definition $\mcG^*$. As we change the group definition keeping $\abs{\mcG}$ constant, the projection of a fixed source distribution $p$ can change. But for all group definitions such that $p \in \skw(\mcG)$, the projection will always be close to some vertex of this simplex.  
\item Now we have set the problem up so that the adversary can pick at least one of the remaining vertices. This is equivalent to saying there is at least one group fully contained in $\Omega_{\theta}(1)$ for some classifier $\theta$. If such a group exits, and our classifier is unfairly-bad on that group, then the adversary can move all the mass to this group, and give us a worst case $q$. This is precisely one vertex of this simplex. The existence of such a \emph{unfairly-bad-minority} group will follow from \emph{Assumption 2} below.
\item Our aim is to argue that under no-regret, $\norm{q(r_t) - u}$ goes to zero with weak conditions on the iterates. That is, we are moving towards learning against the uniform distribution.
\item We can project $\eps(\lt)$ and $\eps(r_t)$ similarly onto the simplex. $\lt$ and $\eps(\lt)$ are vectors in $[0, 1]^{\abs{\mcG}}$ (after relaxation). Similarly the distributions $q(r_t)$ are vectors over this simplex. All group shifts are on this simplex.
\end{itemize}

\emph{Assumption 2: Risk minimization is fair on sufficiently large groups.} That is, there exists an $0.5 < M < 1$ such that, for any $\mcG$ if $p(G_i) \ge M$, 
\[
    \fr(l_{\theta_p}, p; \mcG) \le \eps_{M}.
\]

We have a $p \in \skw(G^*)$. Consider the case when there is only one $G_i$ such that $p(G_i) \le m_1$.

\begin{itemize}
\item Worst case group distribution from $p$ moves all the mass to the $G_i$ that ${\lt}_{p}$ is most \emph{unfairly-bad} on (classifier $\theta_p$ is most unfairly-bad on). If we are already fair on all groups we are done. (We need to be able to detect this -- Not clear yet).
\item If there is an unfairly bad group for ${\lt}_{p   }$, this necessarily is a minority group contained entirely in $\Omega_{{\lt}_p}(1)$. 
\end{itemize}

Main arguments - 1: 
- consider there is only one minority group
- We got skewed $p$. Player one learnt (ideally) $\lt_{p}$. Since there is only one minority group, that is the only group we are un-fair on.


\textbf{Notes:}

Regarding point 1.

More rigorously, we can argue that if $\abs{m_0 - m_1}$ is controlled, i.e. all groups are roughly the same size (even though they are small), the distribution $p$ is already close to uniform over this group distribution. From assumption 1, this implies that we are already fair. How fair we are probably scales like $(\abs{m_0 - m_1})$ since linear.

Regarding point 3

I just want the uniform distribution on to be part of $U_f(p, \delta, \mcG)$, but to be honest, if we keep $\delta$ small for an already skewed distribution, then its easy to show that the worst case $\sup_{q \in U_f(p, \delta, \mcG)} D_f(q\mid p)$ is small for small $\abs{\mcG}$. We are essentially solving a low dim problem. But I also feel that $\delta =1$ is meaningful. 

If you dont agree, we can work with arbitrary $\delta$. THe argument would essentialy be the same but now the equilibrium point is not a point but can be any point on a circle around uniform. We can show that we will be the best among these but it is annoying convex analysis.

Don't need assumption two based on new method.

Regarding assumption 2.

The 0.5 number is not needed. But for now it will make life easier as it ensures there is only 1 majority group for any $\mcG$. This also is our implicitly definition for what it means for a classifier to be fair on a group $G_i \in \mcG$ under a distribution $p$.

TODO: Make sure you are consistent with monotonicity argument as long as $p \in \skw(G^*)$. 
}% subsection - regret results







\clearpage
\section{Can Bitrate DRO robustify last layer re-training?}

\section{Understanding bitrate-constraint (toy)}


\begin{figure}[!h]
\centering
\begin{subfigure}[b]{0.6\textwidth}
    \centering
    \includegraphics[width=\linewidth]{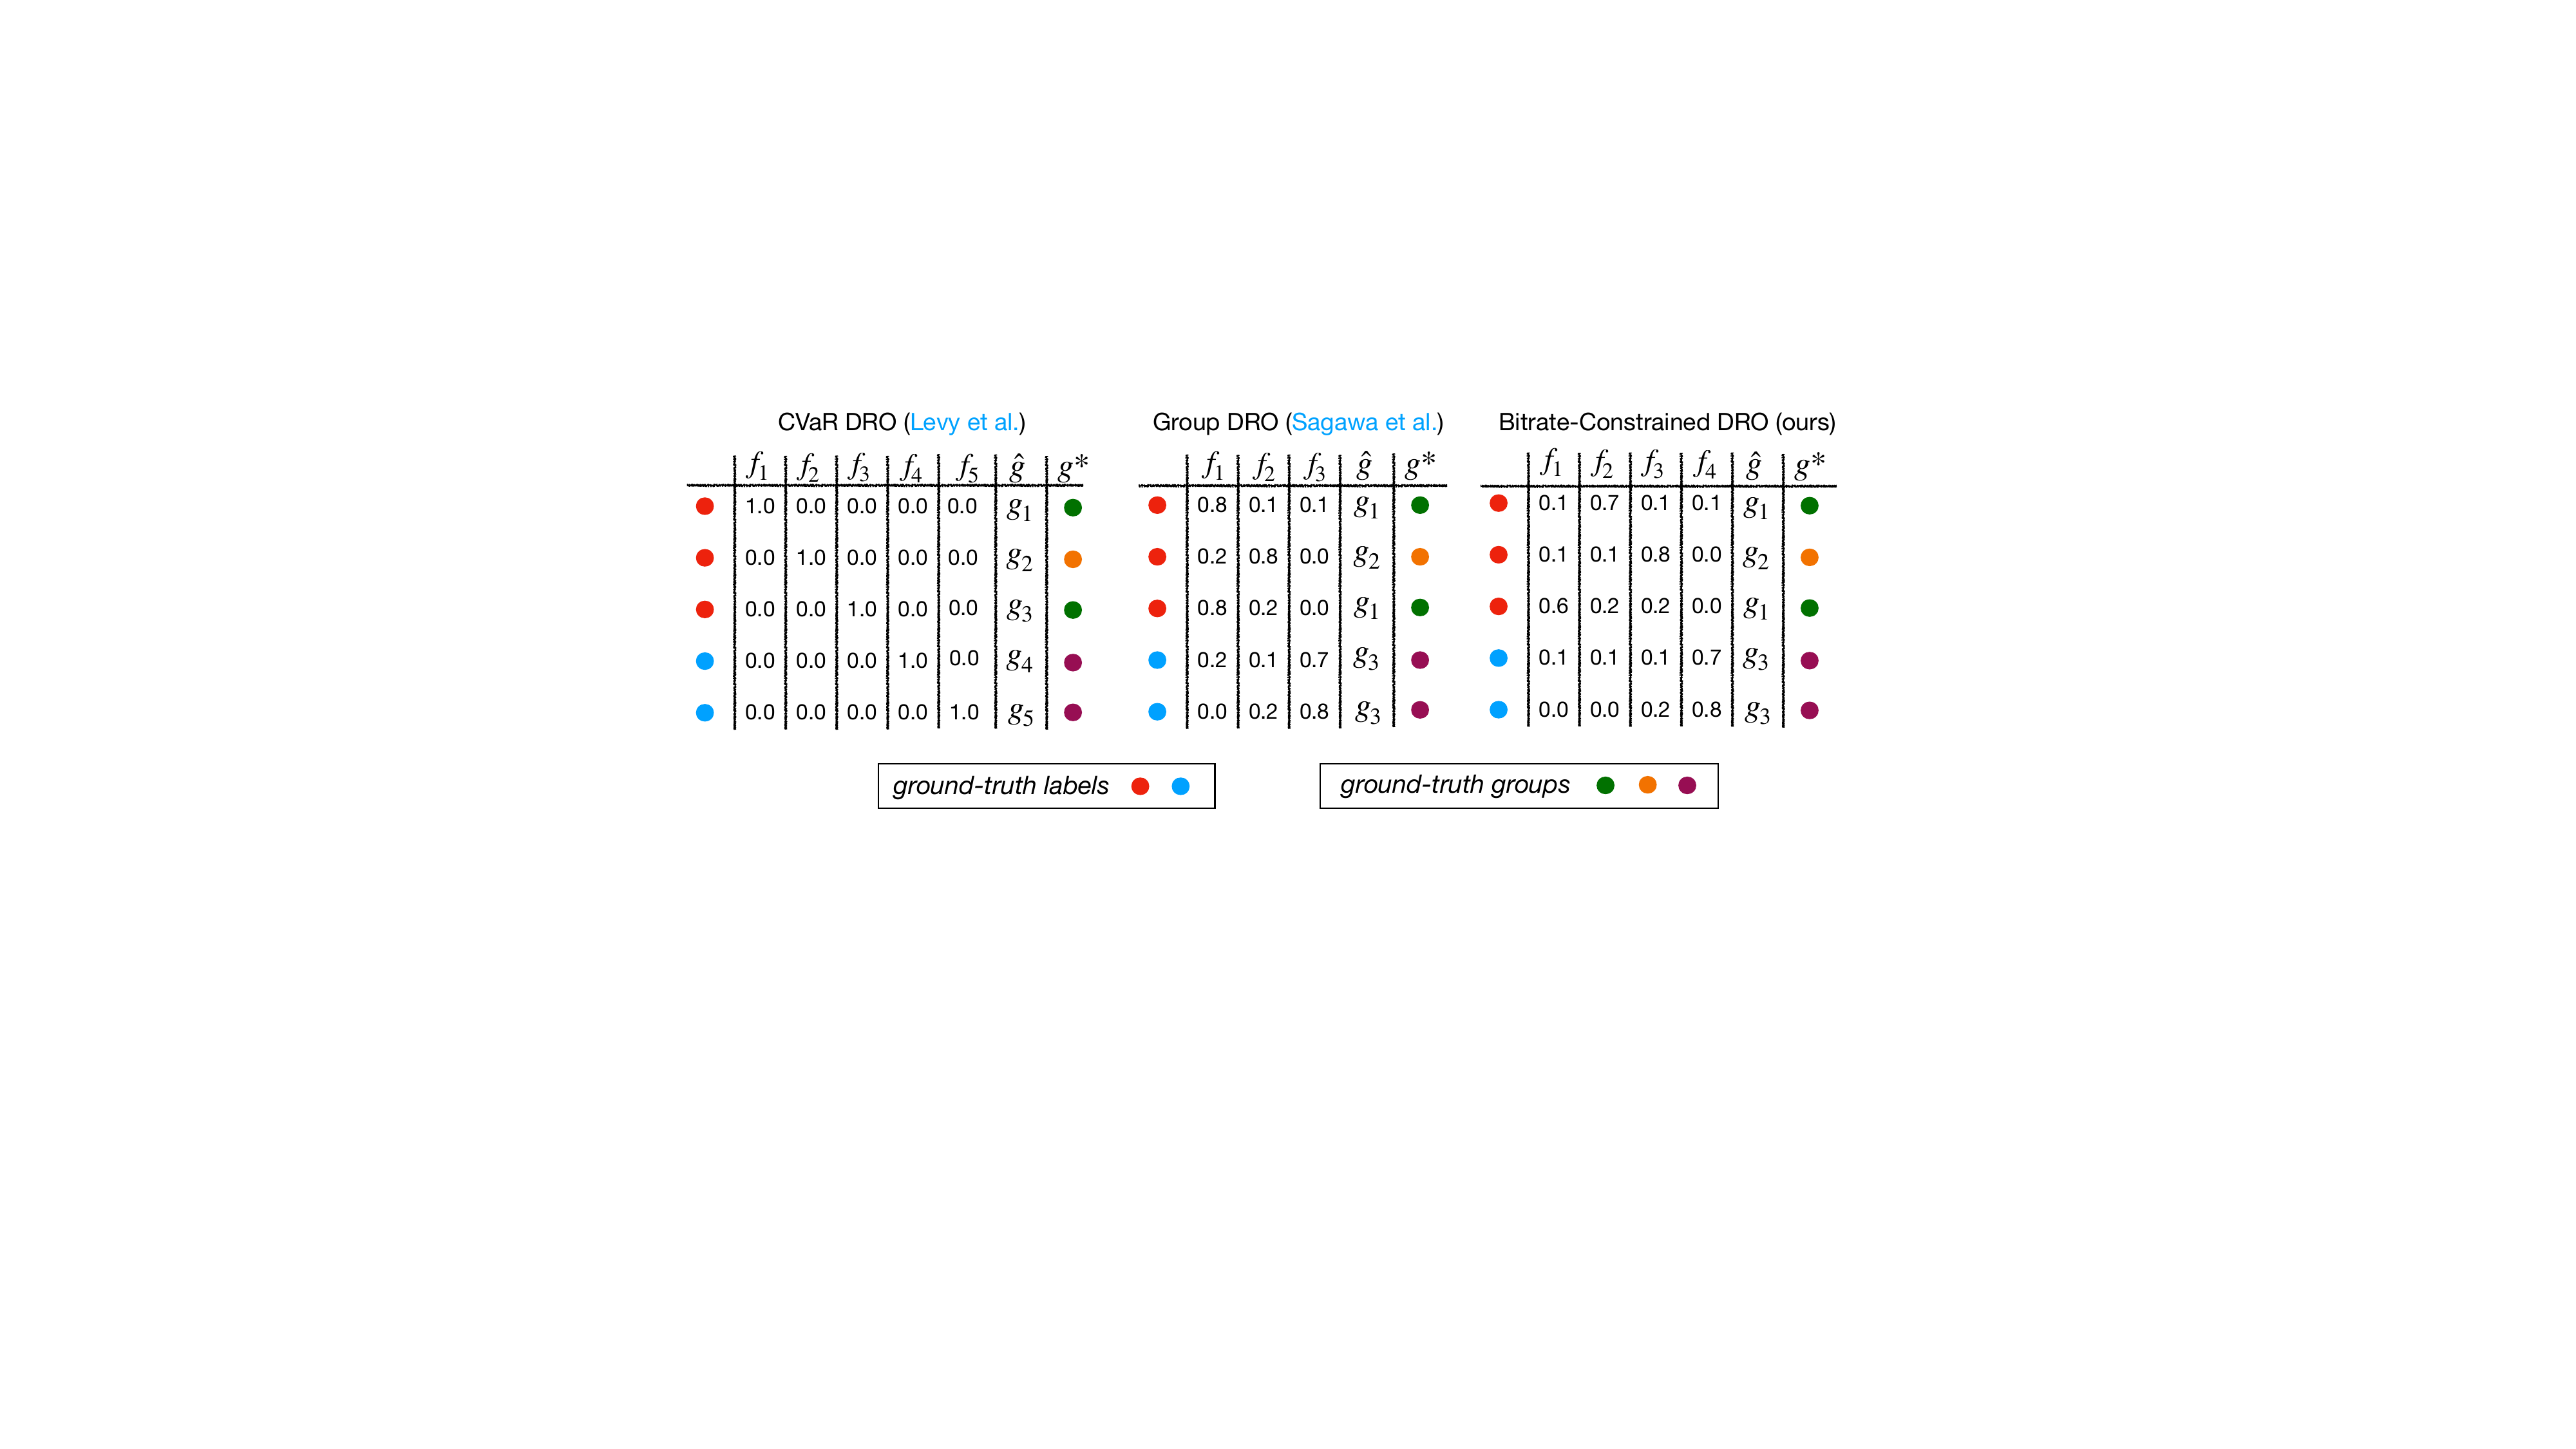}
    \caption{\label{fig:feature-matrix}}
  \end{subfigure} 
\caption{
TBD.
 }
\end{figure}

\begin{table}[!ht]
    \footnotesize
    \centering
    \begin{tabular}{r|cccccc}
         Method & \multicolumn{2}{c}{Waterbirds} & \multicolumn{2}{c}{CelebA} & \multicolumn{2}{c}{CivilComments}   \\ 
                & Avg  & WG & Avg  & WG & Avg & WG \\ \midrule
            ERM                              & 97.2 (0.1) & 72.7 (0.2) & 95.8 (0.2) & 46.9 (0.1) & 92.6 (0.2) & 57.4 (0.2) \\ \midrule
            JTT ~\cite{liu2021just}          & 93.4 (0.2) & \textbf{86.8 (0.3)} & \textbf{87.6 (0.2)} & \textbf{81.3 (0.3)} & 91.0 (0.3) & \textbf{69.2 (0.3)} \\
            Ltf ~\cite{nam2020learning}      & 91.2 (0.1) & 78.0 (0.2) & 85.0 (0.2) & 76.8 (0.3) & 92.1 (0.3) & 58.9 (0.3) \\
            CVaR DRO ~\cite{levy2020large}   & 96.1 (0.2) & 75.9 (0.3) & 82.4 (0.4) & 64.7 (0.2) & \textbf{92.3 (0.4)} & 60.7 (0.3) \\
            SUBY ~\cite{idrissi2022simple}   & 93.7 (0.3) & 82.4 (0.4) & 84.9 (0.1) & 79.9 (0.2) & 91.7 (0.2) & 53.8 (0.3) \\
            Bitrate DRO                      & \textbf{96.5 (0.2)} & \textbf{87.0 (0.3)} & 87.3 (0.1) & \textbf{81.2 (0.2)} & \textbf{92.4 (0.1)} & \textbf{69.4 (0.2)} \\ \midrule
Group DRO ~\cite{sagawa2019distributionally} & 93.2 (0.4) & 91.7 (0.3) & 92.9 (0.2) & 88.5 (0.3) & 88.7 (0.2) & 70.3 (0.3)               
    \end{tabular}
    \vspace{1em}
    \caption{\textbf{Test performance when only re-training the last layer:} on Waterbirds, CelebA and CivilComments. We report both average and worst group accuracy on the test set with each evaluation averaged over $10$ independent runs ($95\%$ confidence interval in $()$).}
    % \label{tab:sc-datasets}
\end{table}


{
\clearpage
\newcommand{\skw}{\Phi} % Skew sets. Need a better notation
\newcommand{\mcG}{\mathcal{G}}
\newcommand{\fr}{\mathcal{F}}
\newcommand{\mcX}{\mathcal{X}}
\newcommand{\lt}{l_{\theta}}
\newcommand{\lth}{{\hat{l}_{\theta}}}
\newcommand{\rth}{{\hat{r}_t}}

\subsection{Regret based stuff}


Main takeaways,
\begin{enumerate}
    \item Fixing a $\abs{\mcG}$, we are robust to all groups of size $\abs{\mcG}$; as robust (fair) as the uniform distribution can be.
    \item We are $O(\sqrt{\frac{\abs{\mcG}}{T}})$ close to optimal $r^*$, not necessarily corresponding to uniform. $r^*$ is implied by the constraint on the adversary. 
    \item In general if $q(r^*) = u + \eps$ for an $\eps$ biased adversarial action space, we are $\eps$ sub-optimal to the most fair classifier (risk minimization against uniform).
    \item Iterate condition option 1 - in case we want more details: Even though our algorithm is playing no-regret sub-optimally, we can still attain $O(\sqrt{T})$-subgradient optimization rate assuming some \emph{weak-learning} like conditions.
    \item All of the above is holds even if we keep on changing $\mcG$ keeping $\abs{\mcG}$ constant \emph{as long as} the adversary is also unbiased on the new action space. Controlling the adversary is critical and if we can't control the adversary uniformly over all $\set{\mcG \mid \abs{\mcG} \text{is fixed}}$, we need to quantify all above statements to all group definitions where we can constrain the adversary. For example, define $\set{\mcG_{\mathcal{A}}}$ where we can constraint the adversary (groups definition based on simple features, say). Then the above is true for all $\mcG$ in this set.
    \item Finally, for high dimensional problems $\abs{\mcG}$, the fair distribution and the `worst adversary' or the most biased adversary (i.e can only play one vertex) differs by $O(1 - \frac{1}{\sqrt{\abs{\mcG}}})$, thus making the solution kind of useless in the worst case. But again, if we have a cooperative or optimistic player 2 (unbiased adversary), we are golden.
    \item \emph{Caution:} Have not thought enough about fairness assumption.
    \item \emph{Caution:} All feelings, no verification.
    \item \emph{Maybe point:} Constraining adversary using bit-rate constraints is one way of ensuring this way of unbaisedness. There could be other ways? In particular, if we know how to construct a constrained adversary for some a set of group definitions $\set{\mcG}$, we can uniformly be as fair (as it gets) to all of them.
    \item (In the general context of any algorithm vs nature) We defined fairness with respect to uniform because we assume nature can uniformly pick over the uncertainty set. Say we want to model some $\pi$ prior for nature instead. We can do that as,
    \[
    \fr(l_\theta, q; \mcG, \pi) = \max_{G_i \in \mcG} \E_\pi\E_{q\mid\pi}[l_{\theta}] - \E_{q\mid G_i}[l_{\theta}].
    \] Setting $\pi = u$ recovers the uniform case where $\E_u \E_{q\mid u} \lt = \E_q \lt$. Moreover, if we want to get the group DRO objective out of this, put the prior on the worst-group ($\pi$ is a vertex of the simplex). Note that the constraint on the adversary also needs to respect the prior.
    
    \item Purity vector -- not $l$ vector. Purity vector is $[0, 1]$ continuous bound and not $\set{0, 1}$. Makes life easier, especially for small $\abs{\mcG}$.
    \item Note that under the uniform assumption you don't even need group information to evaluate unseen distribution performance. It will be, by definition, close to your test performance. Obviously if your test performance it self is garbage there is nothing much we can do.
    
    \item BTW, the intuition for why the dimensional dependency is $\abs{G}$ is the same as why we have a $\sqrt{k}$-separation dependency $k$-means problem in $d$ dimensions, with $d \gg k$. You'd expect a $\sqrt{d}$ separation requirement, say between two gaussians in $d$ dimension, since the gaussian annulus is concentrated at $\sqrt{d}$.  Essentially, the intuition is that the problem is unchanged under a projection onto $\abs{\mcG}$ dimension. See later \url{https://arxiv.org/abs/1206.3204}. 
\end{enumerate}

(Language will be fixed later. Arguments need work)

Notation: 
\begin{itemize}
    \item Speaking mostly on function space over $\mcX$.
    \item $l_\theta : \mcX \rightarrow \set{0, 1}$, will be loss functions indexed by model parameters $\theta \in \Theta$.
    \item $\Delta(\mcX):$ Simplex over $\mcX$, distributions over $\mcX$.
    \item $p, q$ distributions in $\Delta(\mcX)$.
    \item \emph{group definition} $\mcG: \set{G_1, \dots, G_{\abs{G}}}$, $\cup_{G_i} = \mcX$, $G_j \cap G_i = \phi $ for $i \ne j$ (partitions).
\end{itemize}

\begin{definition}[Skew distributions] For a group definition $\mcG = \set{G_1, \dots, G_{\abs{\mcG}}}$, define  
\[
    \mathrm{\skw}(\mcG; m_0, m_1, M)
    = \set{q \in \Delta(\mcX)\mid 0 < m_0 \le q(G_i) \le m_1 \ \text{or}\ q(G_i) > M \ge 0.5, \forall G_i \in \mcG}.
\]
\end{definition}

\begin{definition}[Fair model] For a group definition $\mcG$, a distribution $q$ and $l_\theta$ a $0$-$1$ loss function realized at $\theta \in \Theta$ define,
\[
    \fr(l_\theta, q; \mcG) = \max_{G_i \in \mcG} \E_{q }[l_{\theta}] - \E_{q\mid G_i}[l_{\theta}]
\]
\end{definition}
\begin{enumerate}
    \item $\fr(\cdot, q; G)$ is convex in $l$ for fixed $q$ and $G$. $l$ is convex relaxation of $\lt \in \set{0,1}$ to $ \lt \in [0, 1]$.
    \item $\fr(l, \cdot; G)$ is concave (linear) in $q$ for fixed $l$ and $G$.
\end{enumerate}

For some $q \in \Delta(\mcX)$ let $l_{\theta_{q}} = \argmin_{\theta \in \Theta}\E_{q}l_{\theta}$, the solution returned by risk minimization if we had access to distribution $q$. In particular let $u$ denote the uniform distribution.

\emph{Assumption 1: Risk minimization is fair given oracle access to $u$.} That is, for all (any) $\mcG$, $q$,
\[
 \fr(l_{\theta_u}, u; \mcG) \le \fr(l_{\theta_q}, q; \mcG).
\]

That is, if I had oracle access to the uniform distribution over $\mcX$, I can  learn the most fair model through risk minimization on $u$ and I'll be done.

Here we have not yet restricted $\fr(l_{\theta_u}, u; \mcG)$ from above so it can be quite bad in general. We just need others to be worse. TODO: Think about this. Is this too strong or reasonable? We can relax this later. At some level this is saying that the unbiased oracle is the \emph{right} oracle.

Now let a $\mcG^*$ be such that  $p \in \skw(\mcG^*; m_0, m_1, M)$. That is, we have received data from some skewed distribution with respect to some group definition (fixed for now).

Define set of group shifts around $p$ with respect to groups $\mcG$,
\[
    U_{f}(p, \delta, \mcG) = \set{q \mid D_{f}(q ||p ) \le \delta, \E_{q\mid G_i}I[G_i] = \E_{p\mid G_i} I[G_i]},
\]

\begin{enumerate}
    \item We are going to assume that there is at least one majority group in $\mcG^*$. 
    \item For any fixed $\abs{\mcG^*}$, any distribution can be projected onto $\Delta^{\abs{\mcG}}$. Note that each every group distribution is in $\abs{\mcG^*}$.
    \item For simplicity assume that $\delta = 1$. This means that the uniform distribution can be represented as a group shift. That is $u \in U_f(p, \delta, \mcG)$.
\end{enumerate}

 If thinking in terms of the re-weighting function $r$, replace $q$ with $q(r)$. We can always recover $q$ from $r$. Consider the following optimization program,

\[
    \min_{\lt \in \Theta} \max_{q \in U_f(p, 1.0, \mcG^*)} \fr(\lt, q; \mcG^*) = V^*
\] It follows from assumption $1$ that, 
$$
   V^* = \fr({\lt}_u, q_u; \mcG^*).
$$

Okay the remaining argument is as follows. We are solving,
\[
    \min_{\lt \in \Theta} \max_{q \in U_f(p, 1.0, \mcG^*)} \fr(\lt, q; \mcG^*) = V^*.
\] We know that $(l_{\theta_u}, u)$ (or $(l_{\theta_u}, u(r))$) is the equilibrium point.
Both $\min$-player and $\max$-player is playing no-regret. For concreteness, say both are running  FTRL with $\ell_2$ regularization (i.e gradient descent not SGD sadly).

Thus, at each round both players play ${\lt}_t$ and $q(r_t)$ where,
\[
    {\lt}_t = \arg\min_{\lt} \sum_{\tau=1}^{t-1} \fr(\lt, q(r_\tau); \mcG^*)\quad\text{and}\quad
    q({r}_t) = \arg\min_{q(r) \in U_f(p, 1, \mcG^*)}  \sum_{\tau=1}^{t-1} \fr({\lt}_{\tau}, q(r); \mcG^*).
\]Note that this corresponds to the descent-ascent update rule (roughly -- not being careful),
\[
    {\lt}_t = {\lt}_{t-1} - \frac{1}{\eta} \partial\sum_{\tau=1}^{t-1} \fr({\lt}_t, q(r_\tau); \mcG^*)\quad\text{and}\quad
    q({r}_t) = q(r_{t-1}) - \partial \sum_{\tau=1}^{t-1} \fr({\lt}_{\tau}, q(r_{t-1}); \mcG^*).
\]


Now of course we cannot solve this optimization over $\theta$ or $r$. Since $\theta$ requires us to solve a non-convex problem and picking $r$ requires access to $u$, which in turn requires access of $(G^*)$.

To try to work around this we are going to model $\lth = \lt + \eps(\lt)$ and $q(\rth) = q(r_t) + \eps(r_t)$. Then we are going to control $\eps(\lt)$, $\eps(r_t)$ and invoke Theorem 5.2 here: \url{https://arxiv.org/pdf/1807.04936.pdf}. We can apply the theorem directly for the max-player; they are linear in $q$ so the gradient is just $\lt$. For the min-player the gradient is not $q(\rth)$ by $q\mid{G_i}(\rth)$ for some $i$ so a little work needs to be done to bound it. I will talk about how we control $\eps(\lt)$ and $\eps(r_t)$ in a bit.

This will help us control iterates ${\lt}_t$ and $q({r}_t)$. Finally we invoke Theorem~9, here \url{http://proceedings.mlr.press/v75/abernethy18a/abernethy18a.pdf}, to complete our argument that $(\overline{\lt}, \overline{q(r_t)})$ is $O(\frac{1}{\sqrt{T}}\abs{\mcG})$-equilibrium point.

\paragraph{Controlling $\eps(\lt)$ and $\eps(r_t)$}

Rough arguments:
\begin{itemize}
\item Project everything onto $\Delta^{\mcG - 1}$ using the group conditional projection with a fixed group definition $\mcG^*$. As we change the group definition keeping $\abs{\mcG}$ constant, the projection of a fixed source distribution $p$ can change. But for all group definitions such that $p \in \skw(\mcG)$, the projection will always be close to some vertex of this simplex.  
\item Now we have set the problem up so that the adversary can pick at least one of the remaining vertices. This is equivalent to saying there is at least one group fully contained in $\Omega_{\theta}(1)$ for some classifier $\theta$. If such a group exits, and our classifier is unfairly-bad on that group, then the adversary can move all the mass to this group, and give us a worst case $q$. This is precisely one vertex of this simplex. The existence of such a \emph{unfairly-bad-minority} group will follow from \emph{Assumption 2} below.
\item Our aim is to argue that under no-regret, $\norm{q(r_t) - u}$ goes to zero with weak conditions on the iterates. That is, we are moving towards learning against the uniform distribution.
\item We can project $\eps(\lt)$ and $\eps(r_t)$ similarly onto the simplex. $\lt$ and $\eps(\lt)$ are vectors in $[0, 1]^{\abs{\mcG}}$ (after relaxation). Similarly the distributions $q(r_t)$ are vectors over this simplex. All group shifts are on this simplex.
\end{itemize}

\emph{Assumption 2: Risk minimization is fair on sufficiently large groups.} That is, there exists an $0.5 < M < 1$ such that, for any $\mcG$ if $p(G_i) \ge M$, 
\[
    \fr(l_{\theta_p}, p; \mcG) \le \eps_{M}.
\]

We have a $p \in \skw(G^*)$. Consider the case when there is only one $G_i$ such that $p(G_i) \le m_1$.

\begin{itemize}
\item Worst case group distribution from $p$ moves all the mass to the $G_i$ that ${\lt}_{p}$ is most \emph{unfairly-bad} on (classifier $\theta_p$ is most unfairly-bad on). If we are already fair on all groups we are done. (We need to be able to detect this -- Not clear yet).
\item If there is an unfairly bad group for ${\lt}_{p   }$, this necessarily is a minority group contained entirely in $\Omega_{{\lt}_p}(1)$. 
\end{itemize}

Main arguments - 1: 
- consider there is only one minority group
- We got skewed $p$. Player one learnt (ideally) $\lt{p}$. Since there is only one minority group, that is the only group we are un-fair on.


\textbf{Notes:}

Regarding point 1.

More rigorously, we can argue that if $\abs{m_0 - m_1}$ is controlled, i.e. all groups are roughly the same size (even though they are small), the distribution $p$ is already close to uniform over this group distribution. From assumption 1, this implies that we are already fair. How fair we are probably scales like $(\abs{m_0 - m_1})$ since linear.

Regarding point 3

I just want the uniform distribution on to be part of $U_f(p, \delta, \mcG)$, but to be honest, if we keep $\delta$ small for an already skewed distribution, then its easy to show that the worst case $\sup_{q \in U_f(p, \delta, \mcG)} D_f(q\mid p)$ is small for small $\abs{\mcG}$. We are essentially solving a low dim problem. But I also feel that $\delta =1$ is meaningful. 

If you dont agree, we can work with arbitrary $\delta$. THe argument would essentialy be the same but now the equilibrium point is not a point but can be any point on a circle around uniform. We can show that we will be the best among these but it is annoying convex analysis.

Don't need assumption two based on new method.

Regarding assumption 2.

The 0.5 number is not needed. But for now it will make life easier as it ensures there is only 1 majority group for any $\mcG$. This also is our implicitly definition for what it means for a classifier to be fair on a group $G_i \in \mcG$ under a distribution $p$.

TODO: Make sure you are consistent with monotonicity argument as long as $p \in \skw(G^*)$. 
}% subsection - regret results
